# Supplementary material for: Assessment of the accuracy of coupled cluster perturbation theory for open-shell systems. II. Quadruples expansions
Source: arXiv:1601.06379 ancillary file (2016-05-16)
Supplement: Supplementary file 1 [file si.pdf]

# Supporting information for: Assessment of the accuracy of coupled cluster perturbation theory for open-shell systems. II. Quadruples expansions

Janus J. Eriksen,[*,†] Devin Matthews,[‡] Poul Jørgensen,[†] and Jürgen Gauss[¶]

*qLEAP Center for Theoretical Chemistry, Department of Chemistry, Aarhus University, DK-8000 Aarhus C, Denmark, The Institute for Computational Engineering and Sciences, The University of Texas at Austin, Austin, Texas 78712, United States, and Institut für Physikalische Chemie, Johannes Gutenberg-Universität Mainz, D-55128 Mainz, Germany*

E-mail: janusje@chem.au.dk

[*]To whom correspondence should be addressed
[†]Aarhus University
[‡]The University of Texas at Austin
[¶]Johannes Gutenberg-Universität Mainz

In the following, results for the recovery of the CCSDTQ–CCSDT correlation energy differences are presented in percentage points with respect to 100% for brevity. Results are reported for mean recoveries ($\Delta$) and mean deviations ($\delta$) as well as standard deviations around the means ($\Delta_{\mathrm{std}}$ and $\delta_{\mathrm{std}}$, respectively).

In all tables, the basis set used is cc-pVDZ, and we note that the frozen-core approximation has been invoked for all the calculations reported herein.

Table S1: Recoveries of CCSDTQ/CCSDT correlation energy differences in percent (%) for an RHF reference.

| Molecule | CCSDT(Q) | ΛCCSDT(Q) | CCSDT(Q–2) | CCSDT(Q–3) | CCSDT(Q–4) | CCSDT(Q–5) | CCSDT(Q–6) |
|---|---|---|---|---|---|---|---|
| $C_2H_2$ | 11.90 | 8.31 | -25.13 | -5.10 | -2.89 | -0.57 | -0.53 |
| $C_2H_4$ | 7.34 | 5.01 | -26.52 | -3.74 | -1.78 | -0.15 | -0.17 |
| $CH_2$ ($^1A_1$) | -16.09 | -18.84 | -38.38 | -13.42 | -5.41 | -2.40 | -1.20 |
| $CH_2O$ | 14.57 | 9.27 | -14.95 | 0.20 | -1.74 | 1.31 | -0.82 |
| CO | 14.79 | 9.46 | -16.69 | 2.62 | -3.96 | 3.12 | -2.36 |
| $CO_2$ | 18.15 | 12.96 | -15.56 | 3.89 | -5.88 | 5.20 | -4.99 |
| $F_2$ | 10.27 | 5.45 | -9.34 | -3.56 | -0.36 | -0.28 | -0.02 |
| $H_2O$ | 6.45 | 5.77 | -10.62 | -1.96 | -0.37 | -0.04 | -0.03 |
| $H_2O_2$ | 10.36 | 7.89 | -11.22 | -2.97 | -0.57 | -0.19 | -0.07 |
| HCN | 16.45 | 12.19 | -18.89 | -4.15 | -2.10 | -0.24 | -0.44 |
| HF | 5.10 | 4.77 | -7.79 | -1.17 | -0.24 | 0.03 | -0.03 |
| HNO | 13.23 | 7.89 | -14.50 | -3.31 | -1.49 | -0.11 | -0.49 |
| HOF | 9.63 | 6.15 | -10.50 | -2.89 | -0.57 | -0.15 | -0.09 |
| $N_2$ | 15.60 | 12.01 | -16.02 | -4.62 | -1.64 | -0.50 | -0.30 |
| $N_2H_2$ | 11.64 | 7.74 | -17.51 | -3.69 | -1.37 | -0.27 | -0.21 |
| $NH_3$ | 4.77 | 3.74 | -17.12 | -3.05 | -0.72 | -0.12 | -0.05 |
| $O_3$ | 26.67 | 12.06 | -13.51 | -3.33 | -4.24 | 2.65 | -4.53 |
| $\Delta$ | 10.64 | 6.58 | -16.72 | -2.96 | -2.08 | 0.43 | -0.96 |
| $\Delta_{std}$ | 8.74 | 7.15 | 7.51 | 3.64 | 1.79 | 1.75 | 1.55 |

Table S2: Recoveries of CCSDTQ/CCSDT correlation energy differences in percent (%) for a UHF reference.

| Molecule | CCSDT(Q) | ΛCCSDT(Q) | CCSDT(Q–2) | CCSDT(Q–3) | CCSDT(Q–4) | CCSDT(Q–5) | CCSDT(Q–6) |
|---|---|---|---|---|---|---|---|
| C | -26.91 | -29.78 | -35.07 | -12.52 | -4.58 | -1.72 | -0.67 |
| CCH | 5.20 | 0.95 | -33.43 | -9.73 | -5.87 | -2.62 | -2.01 |
| CF | 15.07 | 1.57 | -17.29 | 4.35 | -4.95 | 4.24 | -4.08 |
| CH | -18.22 | -20.53 | -38.11 | -13.60 | -5.24 | -2.22 | -1.04 |
| $CH_2$ ($^3B_1$) | -12.10 | -13.51 | -29.38 | -8.05 | -2.40 | -0.76 | -0.27 |
| $CH_3$ | -4.05 | -4.76 | -30.68 | -6.87 | -1.92 | -0.49 | -0.15 |
| CN | 41.45 | 18.51 | -27.14 | -1.73 | -4.23 | 1.64 | -1.46 |
| F | -4.32 | -4.99 | -11.21 | -1.95 | -0.31 | -0.07 | -0.02 |
| HCO | 19.56 | 9.88 | -14.26 | 2.40 | -2.45 | 2.64 | -1.55 |
| $HO_2$ | 14.14 | 6.51 | -13.13 | -2.01 | -0.94 | 0.18 | -0.24 |
| N | -22.10 | -23.80 | -24.75 | -6.54 | -1.82 | -0.54 | -0.18 |
| NH | -12.58 | -14.37 | -23.24 | -5.82 | -1.59 | -0.46 | -0.15 |
| $NH_2$ | -2.83 | -4.28 | -19.90 | -4.29 | -1.06 | -0.25 | -0.08 |
| NO | 17.06 | 10.23 | -13.47 | -0.96 | -1.52 | 0.92 | -0.57 |
| O | -12.69 | -13.78 | -18.09 | -3.86 | -0.88 | -0.22 | -0.06 |
| $O_2$ | 10.30 | 7.53 | -11.71 | -4.68 | -0.88 | -0.59 | -0.16 |
| OF | 22.29 | 5.11 | -12.34 | 0.07 | -1.33 | 1.28 | -0.79 |
| OH | -3.74 | -4.83 | -15.09 | -2.89 | -0.66 | -0.13 | -0.05 |
| $\Delta$ | 1.72 | -4.09 | -21.95 | -4.46 | -2.47 | 0.06 | -0.79 |
| $\Delta_{std}$ | 18.46 | 13.48 | 9.00 | 4.87 | 1.78 | 1.71 | 1.04 |

Table S3: Recoveries of CCSDTQ/CCSDT correlation energy differences in percent (%) for an ROHF reference.

| Molecule | ΛCCSDT(Q) | CCSDT(Q–2) | CCSDT(Q–3) | CCSDT(Q–4) | CCSDT(Q–5) | CCSDT(Q–6) |
|---|---|---|---|---|---|---|
| C | -29.91 | -35.58 | -13.26 | -5.42 | -2.60 | -1.57 |
| CCH | 7.59 | -24.87 | -4.06 | -1.27 | 1.22 | 1.26 |
| CF | 1.53 | -17.44 | 4.58 | -5.00 | 4.51 | -4.13 |
| CH | -20.08 | -37.21 | -12.50 | -4.09 | -1.06 | 0.12 |
| $CH_2$ ($^3B_1$) | -13.35 | -29.30 | -8.04 | -2.42 | -0.81 | -0.33 |
| $CH_3$ | -4.66 | -30.72 | -6.90 | -1.97 | -0.55 | -0.21 |
| CN | 16.23 | -19.25 | 2.52 | -2.52 | 4.56 | -1.08 |
| F | -4.88 | -10.77 | -1.47 | 0.18 | 0.42 | 0.47 |
| HCO | 9.55 | -14.85 | 1.99 | -3.33 | 2.13 | -2.46 |
| $HO_2$ | 6.56 | -13.16 | -1.90 | -0.95 | 0.24 | -0.25 |
| N | -24.48 | -25.26 | -7.11 | -2.38 | -1.09 | -0.71 |
| NH | -13.93 | -22.60 | -5.15 | -0.93 | 0.20 | 0.51 |
| $NH_2$ | -4.25 | -19.54 | -3.92 | -0.70 | 0.11 | 0.28 |
| NO | 10.44 | -13.44 | -1.31 | -1.94 | 0.60 | -1.00 |
| O | -13.75 | -17.36 | -3.01 | 0.00 | 0.66 | 0.82 |
| $O_2$ | 11.14 | -7.00 | -1.06 | 3.35 | 3.40 | 4.00 |
| OF | 4.82 | -12.55 | -0.01 | -1.62 | 1.18 | -1.07 |
| OH | -4.67 | -14.73 | -2.53 | -0.29 | 0.23 | 0.32 |
| $\Delta$ | -3.61 | -20.64 | -3.56 | -1.82 | 0.77 | -0.31 |
| $\Delta_{std}$ | 13.72 | 8.77 | 4.91 | 2.08 | 1.95 | 1.71 |

Table S4: Deviations from CCSDTQ correlation energies (in kcal/mol) for an RHF reference.

| Molecule | CCSDT(Q) | ΛCCSDT(Q) | CCSDT(Q–2) | CCSDT(Q–3) | CCSDT(Q–4) | CCSDT(Q–5) | CCSDT(Q–6) |
|---|---|---|---|---|---|---|---|
| $C_2H_2$ | -0.07 | -0.05 | 0.14 | 0.03 | 0.02 | 0.00 | 0.00 |
| $C_2H_4$ | -0.03 | -0.02 | 0.10 | 0.01 | 0.01 | 0.00 | 0.00 |
| $CH_2$ ($^1A_1$) | 0.02 | 0.02 | 0.04 | 0.02 | 0.01 | 0.00 | 0.00 |
| $CH_2O$ | -0.08 | -0.05 | 0.08 | 0.00 | 0.01 | -0.01 | 0.00 |
| CO | -0.09 | -0.06 | 0.10 | -0.02 | 0.02 | -0.02 | 0.01 |
| $CO_2$ | -0.20 | -0.14 | 0.17 | -0.04 | 0.06 | -0.06 | 0.05 |
| $F_2$ | -0.10 | -0.05 | 0.09 | 0.03 | 0.00 | 0.00 | 0.00 |
| $H_2O$ | -0.02 | -0.02 | 0.03 | 0.01 | 0.00 | 0.00 | 0.00 |
| $H_2O_2$ | -0.08 | -0.06 | 0.09 | 0.02 | 0.00 | 0.00 | 0.00 |
| HCN | -0.13 | -0.09 | 0.15 | 0.03 | 0.02 | 0.00 | 0.00 |
| HF | -0.01 | -0.01 | 0.02 | 0.00 | 0.00 | 0.00 | 0.00 |
| HNO | -0.12 | -0.07 | 0.13 | 0.03 | 0.01 | 0.00 | 0.00 |
| HOF | -0.08 | -0.05 | 0.09 | 0.02 | 0.00 | 0.00 | 0.00 |
| $N_2$ | -0.14 | -0.11 | 0.15 | 0.04 | 0.01 | 0.00 | 0.00 |
| $N_2H_2$ | -0.08 | -0.06 | 0.13 | 0.03 | 0.01 | 0.00 | 0.00 |
| $NH_3$ | -0.01 | -0.01 | 0.03 | 0.01 | 0.00 | 0.00 | 0.00 |
| $O_3$ | -0.88 | -0.40 | 0.45 | 0.11 | 0.14 | -0.09 | 0.15 |
| $\delta$ | -0.12 | -0.07 | 0.12 | 0.02 | 0.02 | -0.01 | 0.01 |
| $\delta_{std}$ | 0.20 | 0.09 | 0.10 | 0.03 | 0.03 | 0.03 | 0.04 |

Table S5: Deviations from CCSDTQ correlation energies (in kcal/mol) for a UHF reference.

| Molecule | CCSDT(Q) | ΛCCSDT(Q) | CCSDT(Q–2) | CCSDT(Q–3) | CCSDT(Q–4) | CCSDT(Q–5) | CCSDT(Q–6) |
|---|---|---|---|---|---|---|---|
| C | 0.005 | 0.005 | 0.006 | 0.002 | 0.001 | 0.000 | 0.000 |
| CCH | -0.030 | -0.006 | 0.195 | 0.057 | 0.034 | 0.015 | 0.012 |
| CF | -0.049 | -0.005 | 0.057 | -0.014 | 0.016 | -0.014 | 0.013 |
| CH | 0.009 | 0.010 | 0.018 | 0.006 | 0.002 | 0.001 | 0.000 |
| $CH_2$ ($^3B_1$) | 0.006 | 0.007 | 0.015 | 0.004 | 0.001 | 0.000 | 0.000 |
| $CH_3$ | 0.003 | 0.004 | 0.023 | 0.005 | 0.001 | 0.000 | 0.000 |
| CN | -0.365 | -0.163 | 0.239 | 0.015 | 0.037 | -0.014 | 0.013 |
| F | 0.003 | 0.004 | 0.008 | 0.001 | 0.000 | 0.000 | 0.000 |
| HCO | -0.114 | -0.058 | 0.083 | -0.014 | 0.014 | -0.015 | 0.009 |
| $HO_2$ | -0.098 | -0.045 | 0.091 | 0.014 | 0.007 | -0.001 | 0.002 |
| N | 0.006 | 0.006 | 0.006 | 0.002 | 0.000 | 0.000 | 0.000 |
| NH | 0.010 | 0.011 | 0.018 | 0.005 | 0.001 | 0.000 | 0.000 |
| $NH_2$ | 0.004 | 0.006 | 0.028 | 0.006 | 0.001 | 0.000 | 0.000 |
| NO | -0.134 | -0.081 | 0.106 | 0.008 | 0.012 | -0.007 | 0.005 |
| O | 0.006 | 0.007 | 0.009 | 0.002 | 0.000 | 0.000 | 0.000 |
| $O_2$ | -0.112 | -0.082 | 0.127 | 0.051 | 0.010 | 0.006 | 0.002 |
| OF | -0.138 | -0.032 | 0.076 | 0.000 | 0.008 | -0.008 | 0.005 |
| OH | 0.006 | 0.008 | 0.024 | 0.005 | 0.001 | 0.000 | 0.000 |
| $\delta$ | -0.058 | -0.024 | 0.065 | 0.009 | 0.009 | -0.002 | 0.004 |
| $\delta_{std}$ | 0.097 | 0.048 | 0.070 | 0.019 | 0.011 | 0.008 | 0.005 |

Table S6: Deviations from CCSDTQ correlation energies (in kcal/mol) for an ROHF reference.

| Molecule | ΛCCSDT(Q) | CCSDT(Q–2) | CCSDT(Q–3) | CCSDT(Q–4) | CCSDT(Q–5) | CCSDT(Q–6) |
|---|---|---|---|---|---|---|
| C | 0.006 | 0.007 | 0.002 | 0.001 | 0.000 | 0.000 |
| CCH | -0.044 | 0.145 | 0.024 | 0.007 | -0.007 | -0.007 |
| CF | -0.005 | 0.057 | -0.015 | 0.016 | -0.015 | 0.014 |
| CH | 0.010 | 0.018 | 0.006 | 0.002 | 0.001 | 0.000 |
| $CH_2$ ($^3B_1$) | 0.007 | 0.015 | 0.004 | 0.001 | 0.000 | 0.000 |
| $CH_3$ | 0.004 | 0.023 | 0.005 | 0.001 | 0.000 | 0.000 |
| CN | -0.140 | 0.166 | -0.022 | 0.022 | -0.039 | 0.009 |
| F | 0.004 | 0.008 | 0.001 | 0.000 | 0.000 | 0.000 |
| HCO | -0.056 | 0.088 | -0.012 | 0.020 | -0.013 | 0.015 |
| $HO_2$ | -0.046 | 0.092 | 0.013 | 0.007 | -0.002 | 0.002 |
| N | 0.006 | 0.007 | 0.002 | 0.001 | 0.000 | 0.000 |
| NH | 0.011 | 0.018 | 0.004 | 0.001 | 0.000 | 0.000 |
| $NH_2$ | 0.006 | 0.028 | 0.006 | 0.001 | 0.000 | 0.000 |
| NO | -0.085 | 0.109 | 0.011 | 0.016 | -0.005 | 0.008 |
| O | 0.007 | 0.009 | 0.001 | 0.000 | 0.000 | 0.000 |
| $O_2$ | -0.130 | 0.081 | 0.012 | -0.039 | -0.040 | -0.047 |
| OF | -0.030 | 0.078 | 0.000 | 0.010 | -0.007 | 0.007 |
| OH | 0.008 | 0.024 | 0.004 | 0.000 | 0.000 | -0.001 |
| $\delta$ | -0.028 | 0.056 | 0.003 | 0.004 | -0.007 | 0.000 |
| $\delta_{std}$ | 0.049 | 0.051 | 0.011 | 0.013 | 0.013 | 0.013 |

Table S7: Deviations from CCSDTQ atomization energies (in kJ/mol) for the closed-shell test set (UHF reference for atoms).

| Molecule | ΛCCSDT(Q) | CCSDT(Q–2) | CCSDT(Q–3) | CCSDT(Q–4) | CCSDT(Q–5) | CCSDT(Q–6) |
|---|---|---|---|---|---|---|
| $C_2H_2$ | 0.244 | -0.547 | -0.103 | -0.062 | -0.011 | -0.012 |
| $C_2H_4$ | 0.122 | -0.349 | -0.038 | -0.020 | 0.000 | -0.002 |
| $CH_2$ ($^1A_1$) | -0.067 | -0.157 | -0.055 | -0.022 | -0.010 | -0.005 |
| $CH_2O$ | 0.270 | -0.290 | 0.022 | -0.036 | 0.033 | -0.019 |
| CO | 0.287 | -0.353 | 0.083 | -0.094 | 0.080 | -0.058 |
| $CO_2$ | 0.675 | -0.615 | 0.204 | -0.263 | 0.242 | -0.229 |
| $F_2$ | 0.250 | -0.309 | -0.132 | -0.012 | -0.011 | -0.001 |
| $H_2O$ | 0.097 | -0.090 | -0.015 | -0.003 | 0.000 | 0.000 |
| $H_2O_2$ | 0.322 | -0.303 | -0.084 | -0.016 | -0.005 | -0.002 |
| HCN | 0.443 | -0.557 | -0.117 | -0.062 | -0.006 | -0.014 |
| HF | 0.064 | -0.046 | -0.006 | -0.002 | 0.001 | 0.000 |
| HNO | 0.359 | -0.495 | -0.113 | -0.054 | -0.003 | -0.019 |
| HOF | 0.253 | -0.288 | -0.085 | -0.017 | -0.005 | -0.003 |
| $N_2$ | 0.512 | -0.559 | -0.162 | -0.059 | -0.018 | -0.011 |
| $N_2H_2$ | 0.288 | -0.479 | -0.098 | -0.038 | -0.007 | -0.006 |
| $NH_3$ | 0.057 | -0.115 | -0.018 | -0.004 | 0.000 | 0.000 |
| $O_3$ | 1.759 | -1.764 | -0.439 | -0.583 | 0.369 | -0.628 |
| $\delta$ | 0.349 | -0.430 | -0.068 | -0.079 | 0.038 | -0.059 |
| $\delta_{std}$ | 0.405 | 0.386 | 0.131 | 0.144 | 0.105 | 0.156 |

Table S8: Deviations from CCSDTQ atomization energies (in kJ/mol) for the closed-shell test set (ROHF reference for atoms).

| Molecule | ΛCCSDT(Q) | CCSDT(Q–2) | CCSDT(Q–3) | CCSDT(Q–4) | CCSDT(Q–5) | CCSDT(Q–6) |
|---|---|---|---|---|---|---|
| $C_2H_2$ | 0.245 | -0.546 | -0.101 | -0.061 | -0.010 | -0.010 |
| $C_2H_4$ | 0.123 | -0.348 | -0.036 | -0.019 | 0.002 | 0.000 |
| $CH_2$ ($^1A_1$) | -0.067 | -0.156 | -0.054 | -0.022 | -0.009 | -0.005 |
| $CH_2O$ | 0.271 | -0.290 | 0.021 | -0.037 | 0.032 | -0.020 |
| CO | 0.288 | -0.354 | 0.082 | -0.095 | 0.079 | -0.059 |
| $CO_2$ | 0.676 | -0.617 | 0.201 | -0.266 | 0.239 | -0.232 |
| $F_2$ | 0.249 | -0.311 | -0.134 | -0.015 | -0.014 | -0.004 |
| $H_2O$ | 0.097 | -0.091 | -0.017 | -0.004 | -0.002 | -0.002 |
| $H_2O_2$ | 0.322 | -0.306 | -0.087 | -0.019 | -0.009 | -0.006 |
| HCN | 0.444 | -0.555 | -0.116 | -0.061 | -0.005 | -0.012 |
| HF | 0.064 | -0.048 | -0.008 | -0.003 | -0.001 | -0.002 |
| HNO | 0.360 | -0.496 | -0.114 | -0.055 | -0.004 | -0.020 |
| HOF | 0.253 | -0.291 | -0.088 | -0.020 | -0.008 | -0.006 |
| $N_2$ | 0.513 | -0.557 | -0.161 | -0.057 | -0.017 | -0.010 |
| $N_2H_2$ | 0.290 | -0.478 | -0.097 | -0.037 | -0.006 | -0.005 |
| $NH_3$ | 0.058 | -0.115 | -0.018 | -0.003 | 0.000 | 0.000 |
| $O_3$ | 1.759 | -1.768 | -0.444 | -0.589 | 0.363 | -0.634 |
| $\delta$ | 0.350 | -0.431 | -0.069 | -0.080 | 0.037 | -0.060 |
| $\delta_{std}$ | 0.405 | 0.387 | 0.131 | 0.145 | 0.104 | 0.158 |

Table S9: Deviations from CCSDTQ atomization energies (in kJ/mol) for the open-shell test set (UHF references).

| Molecule | ΛCCSDT(Q) | CCSDT(Q–2) | CCSDT(Q–3) | CCSDT(Q–4) | CCSDT(Q–5) | CCSDT(Q–6) |
|---|---|---|---|---|---|---|
| CCH | 0.069 | -0.762 | -0.218 | -0.136 | -0.061 | -0.048 |
| CF | 0.060 | -0.176 | 0.075 | -0.063 | 0.060 | -0.055 |
| CH | -0.018 | -0.048 | -0.017 | -0.007 | -0.003 | -0.002 |
| $CH_2$ ($^3B_1$) | -0.006 | -0.035 | -0.007 | -0.002 | 0.000 | 0.000 |
| $CH_3$ | 0.008 | -0.070 | -0.012 | -0.003 | 0.000 | 0.000 |
| CN | 0.731 | -0.947 | -0.047 | -0.151 | 0.062 | -0.053 |
| HCO | 0.292 | -0.284 | 0.076 | -0.055 | 0.066 | -0.037 |
| $HO_2$ | 0.246 | -0.308 | -0.043 | -0.024 | 0.006 | -0.007 |
| NH | -0.021 | -0.049 | -0.012 | -0.003 | -0.001 | 0.000 |
| $NH_2$ | 0.001 | -0.089 | -0.018 | -0.004 | -0.001 | 0.000 |
| NO | 0.391 | -0.380 | -0.017 | -0.046 | 0.031 | -0.019 |
| $O_2$ | 0.398 | -0.458 | -0.197 | -0.037 | -0.026 | -0.007 |
| OF | 0.176 | -0.248 | 0.016 | -0.032 | 0.034 | -0.020 |
| OH | -0.004 | -0.065 | -0.012 | -0.003 | 0.000 | 0.000 |
| $\delta$ | 0.166 | -0.280 | -0.031 | -0.040 | 0.012 | -0.018 |
| $\delta_{std}$ | 0.223 | 0.281 | 0.083 | 0.049 | 0.036 | 0.021 |

Table S10: Deviations from CCSDTQ atomization energies (in kJ/mol) for the open-shell test set (ROHF references).

| Molecule | ΛCCSDT(Q) | CCSDT(Q–2) | CCSDT(Q–3) | CCSDT(Q–4) | CCSDT(Q–5) | CCSDT(Q–6) |
|---|---|---|---|---|---|---|
| CCH | 0.231 | -0.551 | -0.078 | -0.023 | 0.034 | 0.033 |
| CF | 0.059 | -0.180 | 0.078 | -0.065 | 0.063 | -0.057 |
| CH | -0.017 | -0.047 | -0.015 | -0.004 | 0.000 | 0.001 |
| $CH_2$ ($^3B_1$) | -0.006 | -0.036 | -0.007 | -0.001 | 0.000 | 0.001 |
| $CH_3$ | 0.009 | -0.069 | -0.011 | -0.002 | 0.000 | 0.001 |
| CN | 0.637 | -0.641 | 0.109 | -0.084 | 0.168 | -0.037 |
| HCO | 0.288 | -0.304 | 0.066 | -0.078 | 0.053 | -0.061 |
| $HO_2$ | 0.248 | -0.314 | -0.043 | -0.028 | 0.004 | -0.011 |
| NH | -0.020 | -0.048 | -0.009 | 0.000 | 0.002 | 0.002 |
| $NH_2$ | 0.002 | -0.087 | -0.015 | -0.001 | 0.002 | 0.002 |
| NO | 0.409 | -0.392 | -0.030 | -0.063 | 0.020 | -0.035 |
| $O_2$ | 0.599 | -0.269 | -0.039 | 0.163 | 0.163 | 0.191 |
| OF | 0.169 | -0.259 | 0.010 | -0.043 | 0.028 | -0.031 |
| OH | -0.003 | -0.064 | -0.011 | -0.002 | 0.000 | 0.000 |
| $\delta$ | 0.186 | -0.233 | 0.000 | -0.017 | 0.038 | 0.000 |
| $\delta_{std}$ | 0.228 | 0.195 | 0.051 | 0.060 | 0.058 | 0.061 |
